# Supplementary material for: Microscopy for Atomic and Magnetic Structures Based on Thermal Neutron Fourier-transform Ghost Imaging
Source: arXiv:1801.10046 ancillary file (2024-03-06)
Supplement: Supplementary file 1 [file supplemental.pdf]

# Calculations on the Scattering of Neutron Field with Arbitrary Incident Wavefront

Kun Chen*

(Dated: January 29, 2018)

* kunchen@siom.ac.cn

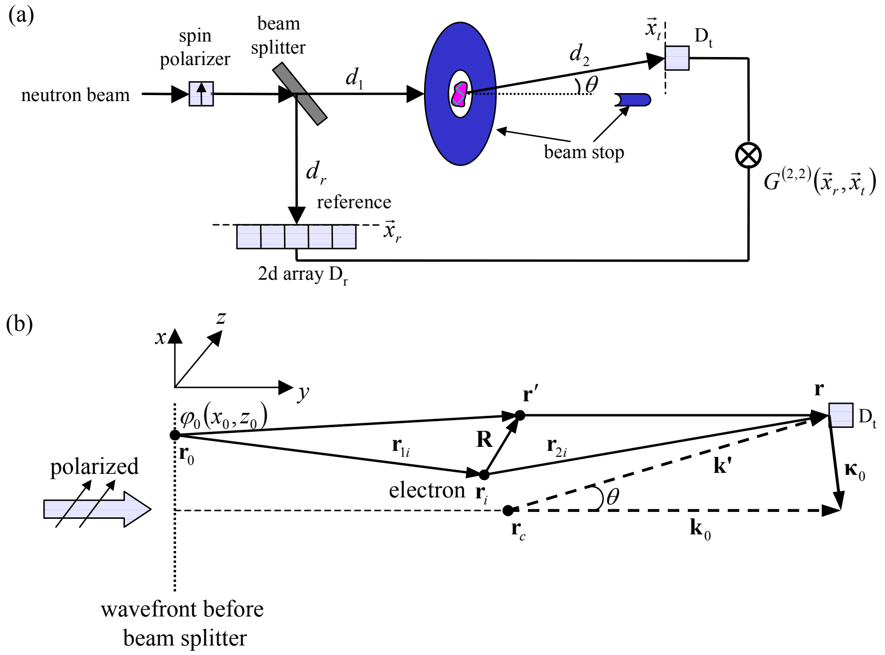


FIG. 1. Illustration of thermal neutron ghost imaging. (a) Schematic experimental setup. A polarized (in $\hat{z}$ dirction), spatially incoherent thermal neutron beam is divided into a sample arm and a reference arm. An extra beam-stop shield is inserted around the sample to remove the incident waves, while the sample is mounted in the opening window of the screen. (b) The definitions of the coordinate system and the vectors used in the calculations, the angles are exaggerated: $\mathbf{r}_0$ one point on the source wavefront, $\mathbf{r}_i$ the $i$-th unpaired electron, $\mathbf{r}$ the detector, $\mathbf{r}'$ a magnetic field point, $\mathbf{r}_c$ the system center.

## I. THE INCIDENT WAVE FUNCTION

Fig. 1 is duplicated from the context of the paper. The incidence plane is set to the plane right at the entrance of the beamsplitter, and the beam is polarized in the $\hat{z}$ direction. The incident wavefront on the incidence plane is described by $\varphi(x_0, z_0)$. This $\varphi(x_0, z_0)$ serves as the source for the incident field of our setup. The Schrödinger equation with this source would be

$$\left(\nabla^2 + k^2\right)\psi(\mathbf{r}) = \rho(\mathbf{r}), \tag{1}$$

where $\rho(\mathbf{r}) = \varphi(x, z)\delta(y - y_0)$. Recall the Green's function for the wave equation

$$\left(\nabla^2 + k^2\right)G(\mathbf{r}, \mathbf{r}') = \delta(\mathbf{r} - \mathbf{r}') \tag{2}$$

is

$$G(\mathbf{r}, \mathbf{r}') = -\frac{\exp(ik\,|\mathbf{r}-\mathbf{r}'|)}{4\pi\,|\mathbf{r}-\mathbf{r}'|}. \tag{3}$$

The incident neutron wave function

$$\psi^{\uparrow}_{\text{in}}(\mathbf{r}) = \frac{1}{i\lambda}\int d\boldsymbol{\eta}\,\varphi(\boldsymbol{\eta})\frac{\exp\left(ik\,|\mathbf{r}-\mathbf{r}_0|\right)}{|\mathbf{r}-\mathbf{r}_0|} \tag{4}$$

is an exact solution to Eq. (1) up to an overall factor. The coefficient has been chosen such that should $\varphi(x_0, z_0) = 1$, the integration would result in $\psi^{\uparrow}_{\text{in}}(\mathbf{r}) = e^{iky}$, a plane wave propagating in the $\hat{y}$ direction. (When carrying out the integration, it has been assumed that $k$ is actually $k + i\epsilon$ with $\epsilon$ a tiny positive number, a common practice as in quantum field theory, which puts $e^{ik\infty}$ to 0.)

$\psi^{\uparrow}_{\text{in}}(\mathbf{r})$ can also be obtained from another point of view. The Schrödinger equation is exactly a wave equation. Neutron wave and optical wave are described by the same mathematical differential equation. Therefore, the Huygens-Fresnel principle in optics also applies to neutrons (see Section 4.1.1, *Statistical Optics*, J. W. Goodman (John Wiley and Sons, New York)), i.e.,

$$\psi^{\uparrow}_{\text{in}}(\mathbf{r}) = \frac{1}{i\lambda}\int d\boldsymbol{\eta}\,\varphi(\boldsymbol{\eta})\frac{\exp\left(ik\,|\mathbf{r}-\mathbf{r}_0|\right)}{|\mathbf{r}-\mathbf{r}_0|}\chi(\Theta), \tag{5}$$

where $\chi(\Theta)$ is an "oblique factor" with the property $\chi(0) = 1$ and $0 \le \chi(\Theta) \le 1$. Because the sample is placed at the $\Theta = 0$ direction, and so is the reference detector after a mirror reflection of the beamsplitter, the "oblique factor" is 1 and Eq. (5) is the same as Eq. (4).

## II. THE SCATTERING WAVE FUNCTION

Consider nucleus $j$ with nuclear spin $I_j$. The neutron spin $\frac{1}{2}\boldsymbol{\sigma}$ and the nuclear spin $I_j$ can form eigenstates $|+\rangle$ and $|-\rangle$ with eigenvalues of total spin $I_j + \frac{1}{2}$ and $I_j - \frac{1}{2}$, respectively. The corresponding free nuclear scattering lengths of $|+\rangle$ and $|-\rangle$ are $b_j^+$ and $b_j^-$ respectively. The operator

$$\hat{b}_j = A_j + B_j\boldsymbol{\sigma}\cdot\mathbf{I}_j, \tag{6}$$

with

$$A_j = \frac{1}{2I_j+1}\left[(I_j+1)b_j^+ + I_j b_j^-\right], \tag{7}$$

$$B_j = \frac{1}{2I_j+1}\left(b_j^+ - b_j^-\right) \tag{8}$$

would take care of all neutron-nuclear spin combinations. Due to the fact that coherent nuclear scattering does not change neutron spin, in this paper we would ignore the $B_j$ term and keep only the $A_j$ term.

Processing the nuclear scattering is straightforward due to the simple form of $\delta$ function. So in the following we would only present calculations on the magnetic scattering. The steps are similar to those in *Introduction to the Theory of Thermal Neutron Scattering*, G. L. Squires (Dover Publications, New York 1996). But details are different due to the double spherical waves in the integrand of Lippmann-Schwinger equation (i.e., spherical wave in and spherical wave out). Therefore, conclusions in conventional neutron literature, derived for plane wave scattering, cannot be directly applied. The original form of magnetic interaction potential from a single unpaired electron at $\mathbf{r}_i$ is

$$V_i^m(\mathbf{r}') = -\frac{\mu_0}{4\pi}\gamma\mu_N 2\mu_B \boldsymbol{\sigma}\cdot\left[\mathbf{W}_{Si}(\mathbf{r}') + \mathbf{W}_{Li}(\mathbf{r}')\right] \tag{9}$$

with

$$\mathbf{W}_{Si}(\mathbf{r}') = \nabla\times\left(\frac{\mathbf{s}_i\times\hat{\mathbf{R}}}{R^2}\right), \tag{10}$$

$$\mathbf{W}_{Li}(\mathbf{r}') = \frac{1}{\hbar}\frac{\mathbf{p}_i\times\hat{\mathbf{R}}}{R^2}, \tag{11}$$

where the Bohr magneton $\mu_B = e\hbar/(2m_e)$, the nuclear magneton $\mu_N = e\hbar/(2m_p)$. Because the neutron mass $m_n$ is very close to the proton mass $m_p$, we can replace one with the other. Taking the definition for the classical radius of electron, $r_e \equiv \mu_0 e^2/(4\pi m_e)$, we simplify Eq. (9) to the form used in the paper

$$V_i^m(\mathbf{r}') = -\frac{\hbar^2}{2m_n}\gamma r_e \boldsymbol{\sigma}\cdot\left[\mathbf{W}_{Si}(\mathbf{r}') + \mathbf{W}_{Li}(\mathbf{r}')\right], \tag{12}$$

Set $\boldsymbol{\eta} = (x_0, z_0)$, from the Lippmann-Schwinger equation the scattering wave function by the single $i$-th electron is

$$\psi^m_{\mathrm{sc},i}(\mathbf{r}) = \frac{\gamma r_e}{4\pi i\lambda}\int d\boldsymbol{\eta}\varphi(\boldsymbol{\eta})\boldsymbol{\sigma}\cdot\int d\mathbf{r}'\frac{\exp\left[ik\left(|\mathbf{r}-\mathbf{r}'|+|\mathbf{r}'-\mathbf{r}_0|\right)\right]}{|\mathbf{r}-\mathbf{r}'|\,|\mathbf{r}'-\mathbf{r}_0|}\left[\mathbf{W}_{Si}(\mathbf{r}') + \mathbf{W}_{Li}(\mathbf{r}')\right]\begin{bmatrix}1\\0\end{bmatrix}. \tag{13}$$

Next we introduce the only assumption in the calculation: the sample size is much smaller than the source-sample distance $d_1$ and the sample-detector distance $d_2$. Though magnetic interaction belongs to the long range category, it is still limited to the local region of the

sample. Let $\mathbf{r}_{1i} = \mathbf{r}_i - \mathbf{r}_0$ and $\mathbf{r}_{2i} = \mathbf{r} - \mathbf{r}_i$, we have $R \ll r_{1i}$ and $R \ll r_{2i}$. Therefore from Fig. 1,

$$|\mathbf{r}' - \mathbf{r}_0| = |\mathbf{r}_{1i} + \mathbf{R}| \approx r_{1i} + \hat{\mathbf{r}}_{1i} \cdot \mathbf{R}, \tag{14}$$

$$|\mathbf{r} - \mathbf{r}'| = |\mathbf{r}_{2i} - \mathbf{R}| \approx r_{2i} - \hat{\mathbf{r}}_{2i} \cdot \mathbf{R}, \tag{15}$$

We further define the scattering vector for the $i$-th electron as $\boldsymbol{\kappa}_i \equiv k(\hat{\mathbf{r}}_{1i} - \hat{\mathbf{r}}_{2i})$. By change the integration variable from $\mathbf{r}'$ to $\mathbf{R}$, Eq. (13) can now be expressed as

$$\begin{aligned}
\psi^m_{\text{sc},i}(\mathbf{r}) &= \frac{\gamma r_e}{4\pi i\lambda} \int d\boldsymbol{\eta}\varphi(\boldsymbol{\eta}) \frac{\exp\left[ik\left(r_{1i} + r_{2i}\right)\right]}{r_{1i} + r_{2i}} \boldsymbol{\sigma} \cdot \int d\mathbf{R} \exp\left(i\boldsymbol{\kappa}_i \cdot \mathbf{R}\right) \left[\mathbf{W}_{Si} + \mathbf{W}_{Li}\right] \begin{bmatrix} 1 \\ 0 \end{bmatrix} \\
&= \frac{\gamma r_e}{i\lambda} \int d\boldsymbol{\eta}\varphi(\boldsymbol{\eta}) \frac{\exp\left[ik\left(r_{1i} + r_{2i}\right)\right]}{r_{1i} + r_{2i}} \boldsymbol{\sigma} \cdot \left[\hat{\boldsymbol{\kappa}}_i \times (\mathbf{s_i} \times \hat{\boldsymbol{\kappa}}_i) + \frac{i}{\hbar\kappa_i} \mathbf{p}_i \times \hat{\boldsymbol{\kappa}}_i\right] \begin{bmatrix} 1 \\ 0 \end{bmatrix}.
\end{aligned} \tag{16}$$

Please refer to Appendix B of *Introduction to the Theory of Thermal Neutron Scattering*, G. L. Squires (Dover Publications, New York 1996) for the $\int d\mathbf{R}\ldots$ integral in Eq. (16).

Let $\mathbf{r}_c$ be the sample center. Again, due to the small sample size condition, we have $|\mathbf{r_i} - \mathbf{r_c}| \ll d_1$ and $|\mathbf{r_i} - \mathbf{r_c}| \ll d_2$. So $\boldsymbol{\kappa}_i \approx \boldsymbol{\kappa}_c$ for all electron sites $i$, where $\boldsymbol{\kappa}_c = k(\hat{\mathbf{r}}_{1c} - \hat{\mathbf{r}}_{2c})$. Sum over all electrons on Eq. (16), we have

$$\psi^m_{\text{sc}}(\mathbf{r}) = \frac{\gamma r_e}{i\lambda} \int d\boldsymbol{\eta}\varphi(\boldsymbol{\eta}) \boldsymbol{\sigma} \cdot \sum_i \frac{\exp\left[ik\left(r_{1i} + r_{2i}\right)\right]}{r_{1i} + r_{2i}} \left[\hat{\boldsymbol{\kappa}}_i \times (\mathbf{s_i} \times \hat{\boldsymbol{\kappa}}_i) + \frac{i}{\hbar\kappa_i} \mathbf{p}_i \times \hat{\boldsymbol{\kappa}}_i\right] \begin{bmatrix} 1 \\ 0 \end{bmatrix}. \tag{17}$$

With the definition for spin magnetization function

$$\mathbf{M}_S(\mathbf{r}') \equiv -2\mu_B \sum_i \delta(\mathbf{r}' - \mathbf{r}_i)\mathbf{s}_i, \tag{18}$$

it is clear the first term in the summation of Eq. (17) is related to

$$\begin{aligned}
\tilde{\mathbf{Q}}_{\perp S}(\mathbf{r}_0, \mathbf{r}) &= -\frac{1}{2\mu_B} \int d\mathbf{r}' \frac{\exp\left[ik(r_1 + r_2)\right]}{r_1 r_2} \hat{\boldsymbol{\kappa}}(\mathbf{r}') \times \left[\mathbf{M}_S(\mathbf{r}') \times \hat{\boldsymbol{\kappa}}(\mathbf{r}')\right] \\
&\approx -\frac{1}{2\mu_B} \int d\mathbf{r}' \frac{\exp\left[ik(r_1 + r_2)\right]}{r_1 r_2} \hat{\boldsymbol{\kappa}}_c \times \left[\mathbf{M}_S(\mathbf{r}') \times \hat{\boldsymbol{\kappa}}_c\right].
\end{aligned} \tag{19}$$

We now consider the communtator

$$\left[\frac{\exp\left[ik\left(r_{1i} + r_{2i}\right)\right]}{r_{1i} r_{2i}}, \mathbf{p}_i\right] = i\hbar\nabla_{\mathbf{r}_i} \left(\frac{\exp\left[ik\left(r_{1i} + r_{2i}\right)\right]}{r_{1i} r_{2i}}\right) \approx -\hbar k \frac{\exp\left[ik\left(r_{1i} + r_{2i}\right)\right]}{r_{1i} r_{2i}} \boldsymbol{\kappa}_i, \tag{20}$$

where as common practice we apply the gradient operator only to the exponential, but not to the denominator; also the relation $k\nabla_{\mathbf{r}_i}(r_{1i}+r_{2i}) = k(\hat{\mathbf{r}}_{1i}-\hat{\mathbf{r}}_{2i}) = \boldsymbol{\kappa}_i$ is used. Because $\boldsymbol{\kappa}_i \times \hat{\boldsymbol{\kappa}}_i = \mathbf{0}$, the second summation term on the r.h.s. of Eq. (17) becomes

$$\begin{aligned}\tilde{\mathbf{Q}}_{\perp L}(\mathbf{r}_0,\mathbf{r}) &\equiv \sum_i \frac{i}{\hbar\kappa_i}\frac{\exp\left[ik\left(r_{1i}+r_{2i}\right)\right]}{r_{1i}r_{2i}}\mathbf{p}_i \times \hat{\boldsymbol{\kappa}}_i \\ &= \sum_i \frac{i}{\hbar\kappa_i}\frac{1}{2}\left[\frac{\exp\left[ik\left(r_{1i}+r_{2i}\right)\right]}{r_{1i}r_{2i}}\mathbf{p}_i + \mathbf{p}_i\frac{\exp\left[ik\left(r_{1i}+r_{2i}\right)\right]}{r_{1i}r_{2i}}\right] \times \hat{\boldsymbol{\kappa}}_i. \qquad (21)\end{aligned}$$

Substituting $\boldsymbol{\kappa}_i \approx \boldsymbol{\kappa}_c$ into the above equation, we have

$$\tilde{\mathbf{Q}}_{\perp L}(\mathbf{r}_0,\mathbf{r}) \approx \frac{i}{\hbar\kappa_c}\left\{\int d\mathbf{r}'\frac{\exp\left[ik(r_1+r_2)\right]}{r_1r_2}\sum_i \frac{1}{2}\left[\delta(\mathbf{r}'-\mathbf{r}_i)\mathbf{p}_i + \mathbf{p}_i\delta(\mathbf{r}'-\mathbf{r}_i)\right]\right\} \times \hat{\boldsymbol{\kappa}}_c, \qquad (22)$$

where $\mathbf{r}_1 \equiv \mathbf{r}' - \mathbf{r}_0$ and $\mathbf{r}_2 \equiv \mathbf{r} - \mathbf{r}'$. In Eq. (22) $r_1$ and $r_2$ no longer contain $\mathbf{r}_i$ and thus commute with $\mathbf{p}_i$, as the dependence on $\mathbf{r}_i$ has been absorbed into the $\delta$ functions. We immediately notice the current operator

$$\mathbf{j}(\mathbf{r}') \equiv -\frac{e}{2m_e}\sum_i \left[\delta(\mathbf{r}'-\mathbf{r}_i)\mathbf{p}_i + \mathbf{p}_i\delta(\mathbf{r}'-\mathbf{r}_i)\right]. \qquad (23)$$

Now Eq. (22) has a much clean form

$$\tilde{\mathbf{Q}}_{\perp L}(\mathbf{r}_0,\mathbf{r}) = -\frac{im_e}{e\hbar\kappa_c}\left\{\int d\mathbf{r}'\frac{\exp\left[ik(r_1+r_2)\right]}{r_1r_2}\mathbf{j}(\mathbf{r}')\right\} \times \hat{\boldsymbol{\kappa}}_c. \qquad (24)$$

Further, we have

$$\mathbf{j}(\mathbf{r}') = \nabla \times \mathbf{M}_L(\mathbf{r}') + \nabla\Phi(\mathbf{r}'), \qquad (25)$$

where $\mathbf{M}_L(\mathbf{r}')$ is interpreted as the current induced magnetization, and $\Phi(\mathbf{r}')$ is an arbitrary scalar function. Both $\mathbf{M}_L(\mathbf{r}')$ and $\Phi(\mathbf{r}')$ vanish at infinity.

Recall that $k\nabla(r_1+r_2) = k(\hat{\mathbf{r}}_1 - \hat{\mathbf{r}}_2) = \boldsymbol{\kappa} \approx \boldsymbol{\kappa}_c$. There exist two relations,

$$\nabla\left[\frac{\exp\left[ik(r_1+r_2)\right]}{r_1r_2}\Phi(\mathbf{r}')\right] \approx \frac{\exp\left[ik(r_1+r_2)\right]}{r_1r_2}\left[\nabla\Phi(\mathbf{r}') + i\Phi(\mathbf{r}')\boldsymbol{\kappa}_c\right], \qquad (26)$$

$$\nabla \times \left[\frac{\exp\left[ik(r_1+r_2)\right]}{r_1r_2}\mathbf{M}_L(\mathbf{r}')\right] \approx \frac{\exp\left[ik(r_1+r_2)\right]}{r_1r_2}\left[\nabla \times \mathbf{M}_L(\mathbf{r}') + i\boldsymbol{\kappa}_c \times \mathbf{M}_L(\mathbf{r}')\right]. \qquad (27)$$

By divergence theorem, the volume integrals of the l.h.s. of Eqs. (26) and (27) become surface integrals over the surface at infinity and thus vanish to 0. Immediately we have

$$\tilde{\mathbf{Q}}_{\perp L}(\mathbf{r}_0,\mathbf{r}) = -\frac{1}{2\mu_B}\int d\mathbf{r}'\frac{\exp\left[ik(r_1+r_2)\right]}{r_1r_2}\hat{\boldsymbol{\kappa}}_c \times \left[\mathbf{M}_L(\mathbf{r}') \times \hat{\boldsymbol{\kappa}}_c\right]. \qquad (28)$$

Substituting Eqs. (19) and (28) into Eq. (17), we arrive at the final result for the magnetic scattering wave function

$$\psi_{\rm sc}^m(\mathbf{r}) = -\frac{\gamma r_e}{2i\lambda\mu_B}\int d\boldsymbol{\eta}\varphi(\boldsymbol{\eta})\boldsymbol{\sigma}\cdot\int d\mathbf{r}'\frac{\exp\left[ik(r_1+r_2)\right]}{r_1 r_2}\hat{\boldsymbol{\kappa}}_c\times\left[\mathbf{M}(\mathbf{r}')\times\hat{\boldsymbol{\kappa}}_c\right], \tag{29}$$

where $\mathbf{M}(\mathbf{r}') = \mathbf{M}_S(\mathbf{r}') + \mathbf{M}_L(\mathbf{r}')$ is the total magnetization function.

## III. PAR-AXIAL APPROXIMATION AND GENERAL EXPRESSION FOR MAGNETIC SAMPLE FUNCTION

Now we discuss the paraxial approximation and the integration leading to the final results. Duplicate from the context of the paper,

$$h_r(\boldsymbol{\xi}_r,\boldsymbol{\eta}) = \frac{e^{ikd_r}}{i\lambda d_r}\exp\left[\frac{i\pi}{\lambda d_r}\left(\boldsymbol{\xi}_r-\boldsymbol{\eta}\right)^2\right]. \tag{30}$$

$$h_t(\boldsymbol{\xi}_t,\boldsymbol{\eta}) = \frac{i}{\lambda}\int d\mathbf{r}'\frac{\exp\left[ik(r_1+r_2)\right]}{r_1 r_2}S(\mathbf{r}'). \tag{31}$$

For a point at $\mathbf{r}' = (x', y', z')$, denote $\boldsymbol{\zeta} = (x', z')$ and we have the following

$$r_1 = |\mathbf{r}'-\mathbf{r}_0| \approx (d_1+y') + \frac{(\boldsymbol{\zeta}-\boldsymbol{\eta})^2}{2d_1}\left(1-\frac{y'}{d_1}+...\right), \tag{32}$$

$$r_2 = |\mathbf{r}-\mathbf{r}'| \approx (d_2-y') + \frac{(\boldsymbol{\xi}_t-\boldsymbol{\zeta})^2}{2d_2}\left(1+\frac{y'}{d_2}+...\right). \tag{33}$$

Small corrections to the denominator of Eq. (31) can be safely ignored and only corrections to the fast varying exponential are important. One nice thing is that the first order corrections due to $y'$ cancel each other in $(r_1+r_2)$. After ignoring higher order corrections, a simpler expression is arrived

$$h_t(\boldsymbol{\xi}_t,\boldsymbol{\eta}) = \frac{i\exp\left[ik(d_1+d_2)\right]}{\lambda}\int d\boldsymbol{\zeta}\frac{\exp\left[\frac{i\pi}{\lambda d_1}\left(\boldsymbol{\zeta}-\boldsymbol{\eta}\right)^2\right]}{d_1}\frac{\exp\left[\frac{i\pi}{\lambda d_2}\left(\boldsymbol{\xi}_t-\boldsymbol{\zeta}\right)^2\right]}{d_2}\int dy' S(\mathbf{r}'). \tag{34}$$

The integration

$$I_0^2\int d\boldsymbol{\eta}h_r^*(\boldsymbol{\xi}_r,\boldsymbol{\eta})h_t(\boldsymbol{\xi}_t,\boldsymbol{\eta})$$

would lead to the result in the paper.

In Fig. 2 the incident $\mathbf{k}_0 = k(0,1,0)$ and the exit $\mathbf{k}' = k(\sin\theta\sin\phi, \cos\theta, \sin\theta\cos\phi)$. Then

$$\hat{\boldsymbol{\kappa}}_0 = \left(-cos\frac{\theta}{2}\sin\phi, \sin\frac{\theta}{2}, -\cos\frac{\theta}{2}\cos\phi\right). \tag{35}$$

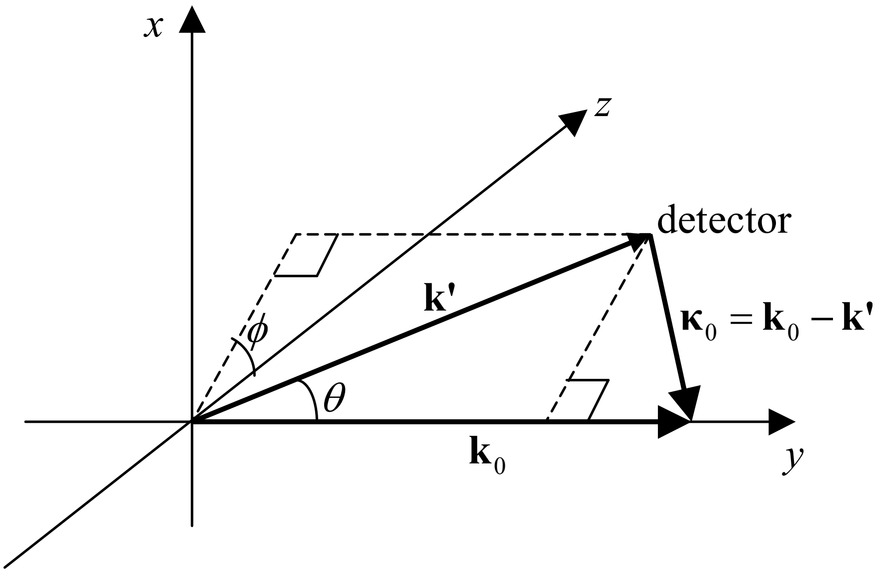


FIG. 2. Definition of the scattering angle $\theta$ and the azimuthal angle $\phi$ around the $y$-axis.

A straightforward calculation presents

$$\begin{aligned}
\mathbf{M}_{\perp} &= \hat{\boldsymbol{\kappa}}_0 \times (\boldsymbol{M} \times \hat{\boldsymbol{\kappa}}_0) = (M_{\perp x}, M_{\perp y}, M_{\perp z}),\\
M_{\perp x} &= M_x\left(1-\cos^2\frac{\theta}{2}\sin^2\phi\right) + \frac{1}{2}M_y\sin\theta\sin\phi - M_z\cos^2\frac{\theta}{2}\sin\phi\cos\phi,\\
M_{\perp y} &= \frac{1}{2}M_x\sin\theta\sin\phi + M_y\cos^2\frac{\theta}{2} + \frac{1}{2}M_z\sin\theta\cos\phi,\\
M_{\perp z} &= -M_x\cos^2\frac{\theta}{2}\sin\phi\cos\phi + \frac{1}{2}M_y\sin\theta\cos\phi + M_z\left(1-\cos^2\frac{\theta}{2}\cos^2\phi\right),
\end{aligned} \tag{36}$$

and the probed sample functions

$$\begin{bmatrix} S^{\uparrow}(\mathbf{r}') \\ S^{\downarrow}(\mathbf{r}') \end{bmatrix} = \{\beta\boldsymbol{\sigma}\cdot[\hat{\boldsymbol{\kappa}}_0 \times (\mathbf{M}(\mathbf{r}') \times \boldsymbol{\kappa}_0)] + A(\mathbf{r}')\} \begin{bmatrix} 1 \\ 0 \end{bmatrix} \tag{37}$$

become

$$S^{\uparrow} = -\beta M_x\cos^2\frac{\theta}{2}\sin\phi\cos\phi + \frac{\beta}{2}M_y\sin\theta\cos\phi + \beta M_z\left(1-\cos^2\frac{\theta}{2}\cos^2\phi\right) + A \tag{38}$$

$$\begin{aligned}
S^{\downarrow} &= \beta M_x\left(1-\cos^2\frac{\theta}{2}\sin^2\phi + \frac{i}{2}\sin\theta\sin\phi\right) + \beta M_y\left(\frac{1}{2}\sin\theta\sin\phi + i\cos^2\frac{\theta}{2}\right)\\
&\quad +\beta M_z\left(-\cos^2\frac{\theta}{2}\sin\phi\cos\phi + \frac{i}{2}\sin\theta\cos\phi\right).
\end{aligned} \tag{39}$$

It is clear Eqs. (38) and (39) can provide different combinations of $M_x$, $M_y$ and $M_z$ by place the detector at different location $(\theta, \phi)$. We would consider a special case when $\theta \to 0$.

Because the incident field is polarized in the $+z$ direction, it is absent in the spin-flip signal $S^{\downarrow}$. However, $S^{\downarrow}$ is not unique when we approach $\theta = 0$ along different $\phi$ angle, i.e.

$$\lim_{\theta \to 0} S^{\downarrow} = \beta M_x \cos^2 \phi + i\beta M_y - \frac{\beta}{2} M_z \sin 2\phi. \tag{40}$$

In real world, this is not a problem because the collecting plane of the detector always has a finite size and the signal is actually the integration over a solid angle. Therefore,

$$\frac{1}{2\pi} \int_0^{2\pi} d\phi \lim_{\theta \to 0} S^{\downarrow} = \frac{\beta}{2} M_x + i\beta M_y. \tag{41}$$

This concludes our calculations.
